# Supplementary material for: Metric Clustering and MST with Strong and Weak Distance Oracles
Source: arXiv:2310.15863 source file (2023-10-24)
Supplement: Supplementary file 1 [file appendixExperiments.tex]

% \section{Additional Details of the Experiments}
% \label{app:experiment}

% % \paragraph{Additional details of the implementation.} 

% \paragraph{Additional experiment results.}
% We present the additional figures of our experiments that we skipped in \Cref{sec:experiment} in this section.
